# Supplementary material for: History matching for functional data: Application to tsunami warnings in the Indian Ocean
Source: arXiv:2509.04342 source file (2026-08-29)
Supplement: Supplementary file 1 [file Supplement.pdf]

# Functional history matching for tsunami warnings: supplemental material

## 1. WORST-CASE SCENARIO TSUNAMI TIME SERIES DATA AND DATA PRE-PROCESSING

This study analyzes the worst-case scenario tsunami that could occur off the Makran coast, as studied in [Gopinathan et al. \(2021\)](#) and described in Fig. S1 and S2. Fig. S2 shows the same tsunami from different angles. As shown in these figures, the rise and fall of the sea level occur simultaneously but have different shapes; they are not mirror images of each other. In addition, each phase, whether rising or falling, has an asymmetric waveform when considered on its own. This waveform asymmetry persists under any time shift or rescaling and cannot be accurately reproduced using a Gaussian shaped waveform. We performed tsunami simulations in this area using the JAGURS simulator ([Baba et al. 2015, 2017](#)). The resolution of both the bathymetry and tsunami input files for the simulation is set to 15 arcseconds. The time step for the tsunami simulation depends on the bathymetry resolution and the maximum seabed depth, as expressed in Equation S1.

$$dt \simeq \frac{\Delta x}{\sqrt{2gh}}, \quad (S1)$$

where  $dt$  is the time resolution (seconds),  $\Delta x$  is the resolution of the bathymetry file (meters),  $g$  is the gravitational acceleration ( $9.8m/s^2$ ), and  $h$  is the maximum depth (meters). For this target area, we confirmed that JAGURS could perform calculations without any problems with  $dt = 1.5$ . Therefore, all calculations were executed with  $dt = 1.5$ .

To apply functional history matching in this study, it is necessary to restrict the time window of the tsunami observations. Analyzing intervals with no sea-level change is not informative, and using the entire observation period would incur unnecessary computational cost. Hence, it is more efficient to analyze a limited range. Therefore, a limited time window was used. As described in the main text, a 30-minute interval was extracted at four DART stations (buoys): DART23228 from 10:30 to 11:00, DART23226 from 10:50 to 11:20, DART23225 from 11:05 to 11:35, and DART23011 from 11:30 to 12:00. In the tsunami simulations, the simulation time step  $dt$  in JAGURS was set to 1.5 s, which yields 1201 samples per 30-minute interval when both endpoints are included. We then downsampled each observed time series by a factor of 12, sampling every twelfth point, to preserve the overall waveform shape, resulting in 101 samples per interval for analysis. For the virtual observation point indicated by a black circle in Figure S1, a 30 minute

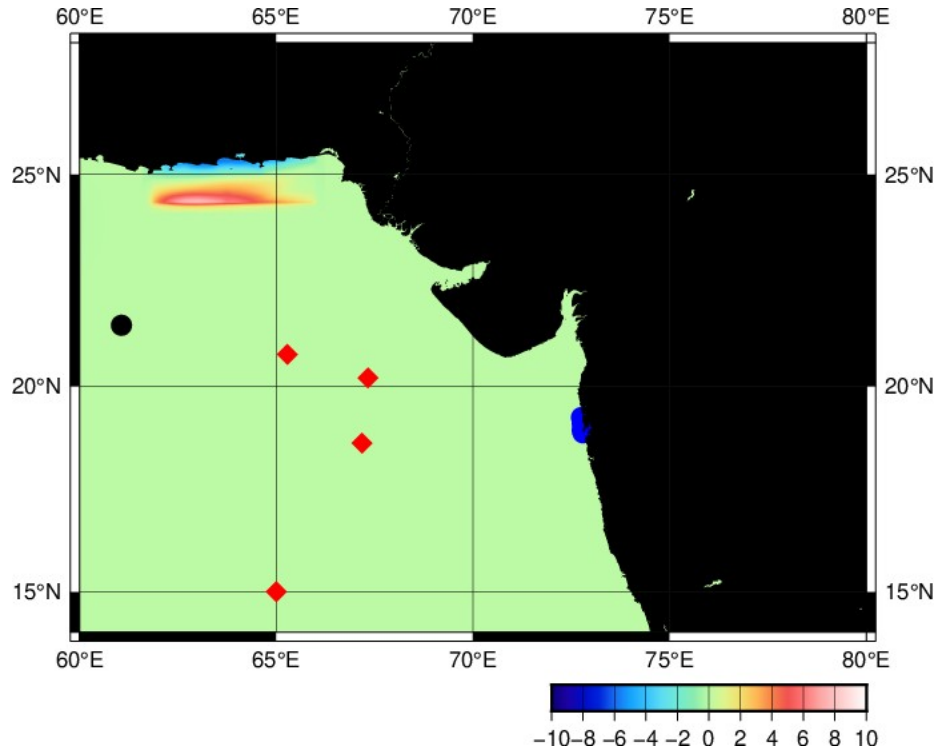

**Fig. S1.** A two-dimensional diagram of a tsunami in a worst-case scenario. Black represents the land, light green represents the sea surface, red indicates sea level rise due to the tsunami, and blue indicates sea level fall caused by the tsunami.

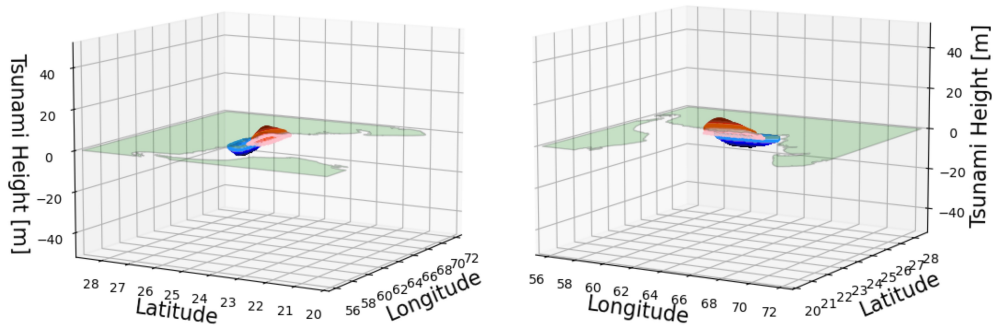

**Fig. S2.** The worst-case scenario tsunami from different angles. The green color represents land, the red color indicates sea level rise, and the blue color represents sea level fall.

interval from 10:30 to 11:00 was extracted and downsampled in the same way, yielding 101 samples for analysis.

For forecasting in Mumbai, we extracted a 90-minute interval from 14:30 to 16:00 at observation points 001 and 002, yielding 3,601 samples per point when both endpoints are included, and a 120-minute interval from 14:00 to 16:00 at observation points 003 and 004, yielding 4,801

samples per point. We then downsampled each time series by a factor of 12, retaining every twelfth point to preserve the overall waveform shape, resulting in 301 samples per point for observation points 001 and 002 and 401 samples per point for observation points 003 and 004. The selected analysis windows for these observation points, the virtual observation point, and the forecast points in Mumbai are shown in Figure 1 in the main paper as shaded and hatched regions. The extracted time series were then represented in functional form using a B-spline basis.

To perform functional emulation using Outer Product Emulator (OPE) (Rougier 2008), it is necessary to determine the correlation lengths  $\lambda_{j_\theta}$  and  $\lambda_t$  for  $\kappa_\lambda^\theta(\theta, \theta')$  and  $\kappa_\lambda^t(t, t')$ , respectively, as defined in Equations 9 and 10 of the main paper. The training data used to construct the emulator comprised the 30-minute intervals described above, which were rescaled to the  $[0, 1]$  range. Similarly, all simulation input parameters (longitudes and latitudes of the rising and falling tsunami centers, standard deviations in the longitude and latitude directions, and the maximum tsunami height) were rescaled to the  $[0, 1]$  range. On this basis, we assumed a uniform correlation length  $\lambda_\theta$  across all parameters and estimated its value. The procedure was as follows. First, we performed five additional tsunami simulations with JAGURS that were not included in the ensemble used to train the emulator. Next, using the input parameter values from these additional simulations, we emulated the corresponding tsunami time series with an OPE trained on the aforementioned ensemble. We then compared the outputs of the JAGURS simulations with those from the OPE emulation. During this process, we considered 50 candidate values for each of  $\lambda_\theta$  and  $\lambda_t$ , ranging from 0.1 to 9.9 in increments of 0.2, and selected the three value pairs that yielded the smallest root mean square error (RMSE) for each tsunami time series. This procedure was applied at each of the four DART observation points. Consequently, a total of 60 value pairs were selected from the 2,500 potential combinations. We then took the average of these selected pairs as the estimates of the correlation lengths  $\lambda_{j_\theta}$  and  $\lambda_t$ . The resulting correlation lengths were as follows: for Wave 1,  $\lambda_\theta = 1.143$  and  $\lambda_t = 1.956$ ; for Wave 2,  $\lambda_\theta = 0.896$  and  $\lambda_t = 1.700$ .

## 2. SENSITIVITY ANALYSIS

To assess the validity of the emulator selected by the RMSE criterion, we conducted a sensitivity analysis. We varied one input parameter at a time while holding the other four fixed and examined the resulting outputs. The sensitivity analysis results at the DART23228 observation point are shown in Figure S3. Varying an input parameter changes the shape of the tsunami time series. However, these changes do not produce qualitatively different waveforms or implausible outputs. These observations provide preliminary evidence that the emulator was constructed successfully. It is important to note, however, that apparent adequacy at this stage does not guarantee that the emulator will reproduce the simulator outputs for arbitrary input settings.

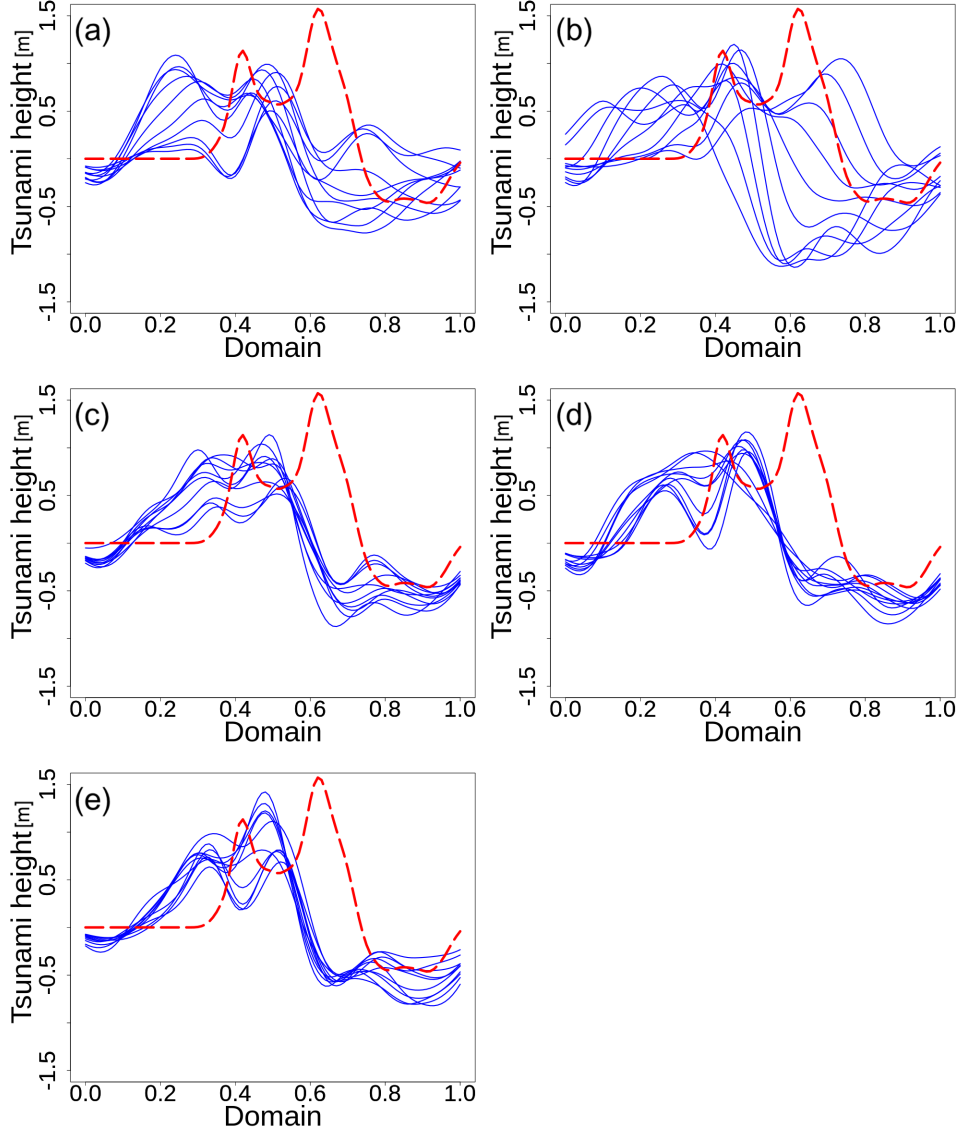

**Fig. S3.** Sensitivity analysis at the location of DART 23228. The worst-case scenario (thick dashed line) and variations of each parameter from their minimum to maximum values at equal intervals, are shown in 10 changes (thin solid lines). The varying parameter in each panel is (a) longitude, (b) latitude, (c)  $S_{xx}$ , (d)  $S_{yy}$ , and (e) the maximum tsunami height, respectively.

Upon further observation of how tsunami time series shapes respond to changes in parameter inputs, it is clear that the latitude parameter causes the most significant alterations in the case of the wave 1 emulator as displayed in Panel (b) in Figure S3. Based on this finding, it is conjectured that the parameter  $\theta_2$  could be reduced relatively more than other parameters in wave 1. The

longitude parameter,  $\theta_1$ , has the second greatest impact on the variability of the emulator output following the latitude parameter. Thus, in wave 1, it is expected that  $\theta_1$  also tends to have a smaller non-implausible region. These inferences can be confirmed as correct by the violin plots of the NROY subspace in Figure 6 of the main paper, which show that the NROY spaces for  $\theta_1$  and  $\theta_2$  are the most reduced. On the other hand, this sensitivity analysis for  $S_{xx}$ ,  $S_{yy}$ , and the tsunami height suggests that the shape changes minimally with variations leading to the hypothesis that the parameter space may not be significantly reduced in direction  $\theta_3$ ,  $\theta_4$ , and  $\theta_5$ . The validity of these conjectures is also confirmed through violin plots of wave 1.

For Wave 2, we build an emulator using a different set of simulation ensembles with input parameter values from  $\Theta_1$ . Consequently, it is presumed that the directions susceptible to reduction in this reduced subspace are different from those in wave 1. The comparison of violin plots from wave 1 and wave 2 allows for the verification of this conjecture.

### 3. DISTANCE EVALUATION BETWEEN FUNCTIONS

The next step in computing implausibility is to evaluate the similarity between the emulated curves and the worst-case tsunami time series. Numerous methods exist for evaluating similarity or distance between functions. Examples include methods for assessing similarity between functions in functional-data clustering (Ferreira & Hitchcock 2009) and for clustering sparsely sampled functional data (James & Sugar 2003). In addition, there are comparative studies of similarity and distance measures (Tokushige et al. 2003). Later work examined preprocessing to improve clustering (Hitchcock et al. 2006) and addressed phase variation (Marron et al. 2015).

#### A. $L_p$ Norm

A basic measure of size for functions is the  $L^p$  norm, defined as follows.

$$\|f\|_p := \left( \int_S |f|^p d\mu \right)^{1/p}, \quad (\text{S2})$$

where  $p = 1, 2, \dots, \infty$ . The induced distance between functions is  $d_p(f, g) = \|f - g\|_p$ . However, in some settings, these norms are not ideal for assessing similarity between functional data. In particular, the  $L_1$  and  $L_2$  norms primarily reflect amplitude differences and do not explicitly account for phase variation. Consequently, they may fail to capture features revealed by derivatives of the functions. They integrate value differences over the domain and can yield unsatisfactory results in the presence of phase variability (Marron et al. 2015). The  $L_\infty$  norm,  $\|f\|_\infty \equiv \inf\{C \geq 0 : |f(x)| \leq C \text{ for almost every } x\}$ , emphasizes the maximum absolute deviation over the domain and does not capture phase variation. Functional data exhibit both amplitude and phase variation, such as changes in peak and trough locations, which are central

to this study. Therefore,  $L_p$  based distances are not well suited to our objectives, which require accounting for phase variation.

## B. Dynamic Time Warping and Fréchet distance

Other techniques include Dynamic Time Warping (DTW) (Sakoe & Chiba 1978) and the Fréchet distance (Alt & Godau 1995), which are widely used for time-series similarity. Both operate on discretized time series: DTW minimizes an alignment cost between two sequences, whereas the Fréchet distance measures the maximum of the shortest distances along an optimal traversal of the curves Brankovic et al. (2020). However, several issues limit their use here. First, tsunami analysis requires real-time processing, yet these methods can be computationally intensive. Second, while DTW aligns sequences by allowing phase shifts, the resulting distance primarily reflects amplitude differences after alignment; quantifying phase similarity would require analyzing the warping function and propagating uncertainty, which is computationally demanding. Similarly, while the Fréchet distance permits monotone time reparameterization, it emphasizes the maximal discrepancy along an optimal traversal and is sensitive to noise and sampling density. Moreover, it does not naturally propagate emulator or observational uncertainty, and its pairwise computational cost is prohibitive in our large scale, near real time setting. Because the goal is timely warning, methods that do not efficiently incorporate peak and trough timing under uncertainty are not aligned with our objectives.

## C. Sobolev Norm

The Sobolev norm provides an alternative that incorporates derivatives up to order  $k$ , not just the first derivative. The Sobolev space  $W^{k,p}$  consists of functions whose derivatives up to order  $k$  lie in  $L^p$  space. For  $p = 2$ ,  $W^{k,2}$  is a Hilbert space  $H^k$  with norm

$$\|f\|_{k,2} := \left( \sum_{i=0}^k \int_{\mathbb{T}} \left| \frac{d^i f(t)}{dt^i} \right|^2 dt \right)^{1/2}. \quad (\text{S3})$$

However, the computational cost of the Sobolev norm is even higher than that of the  $L_2$  norm, and as the degree of differentiation  $k$  increases, the Sobolev norm value also continues to increase, making it difficult to handle. In our setting, distances feed into the implausibility calculation in Equation 1 of the main paper to separate implausible from non-implausible regions. The purpose is then to use the calculated implausibility to separate the implausible and non-implausible parameter subspace based on a certain threshold. Changing  $k$  alters the norm and can shift threshold based decisions, risking misclassification of regions. Because we lack a principled and computationally feasible rule for choosing  $k$ , and decisions are sensitive to this choice, Sobolev based distances are not well suited to our screening objective.

#### D. Functional Principal Component Analysis

Another approach is to project functional data and compare distances between the resulting scores. We consider functional principal component analysis (FPCA) ([Ramsay & Silverman 2005](#)), a standard tool in functional data analysis. As discussed in the main paper, FPCA alone is inadequate for our objective. Let  $X(t) \in L^2[0, 1]$  with mean

$$\mu(t) = E[X(t)] \quad (\text{S4})$$

and covariance

$$\Gamma(s, t) = \text{Cov}(X(s), X(t)) \quad (\text{S5})$$

Then, the covariance operator can apply to functions  $f(t)$  in  $L^2[0, 1]$ .

$$(\Gamma f)(t) = \int_{s \in [0, 1]} f(s) \Gamma(t, s) ds \quad (\text{S6})$$

Given the continuity of  $\Gamma(s, t)$ , the covariance function can be expressed as follows.

$$\Gamma(s, t) = \sum_{j=1}^{\infty} \xi_j \psi_j(s) \psi_j(t), \quad (\text{S7})$$

where  $\xi_j$  and  $\psi_j$  are eigenvalues and eigenfunctions satisfying  $\Gamma \psi_j = \xi_j \psi_j$ . It should be noted that  $\xi_j$  are arranged in descending order. In this case, through the Karhunen-Loève expansion ([Loeve 1948](#), [Karhunen 1947](#)), the difference between  $X_i$  and the mean function can be represented as below.

$$X_i(t) - \mu(t) = \sum_{j=1}^{\infty} \zeta_{ij} \psi_j(t), \quad (\text{S8})$$

$$\zeta_{ij} = \int_{t \in [0, 1]} (X_i(t) - \mu(t)) \psi_j(t) dt \quad (\text{S9})$$

Also, the mean and the variance of  $\zeta_{ij}$  are represented as  $E[\zeta_{ij}] = 0$  and  $\text{Var}[\zeta_{ij}] = \xi_j$ , respectively ([Hall et al. 2006](#)). This expansion is also referred to as the functional principal component expansion.

For comparison, we applied the following FPCA based procedure. First, following our functional history matching procedure, we sampled 100 parameter settings using Latin hypercube sampling and ran the corresponding JAGURS simulations with those settings. Next, we trained an OPE based emulator on this ensemble, then generated 1,000,000 distinct input settings by Latin hypercube sampling and evaluated the emulator at each DART point, yielding one million emulated time series per point. We then applied FPCA to the emulated curves and the worst-case scenario curve, obtaining principal component scores for each principal direction and the contribution of each principal component. At DART23228, the first two principal components



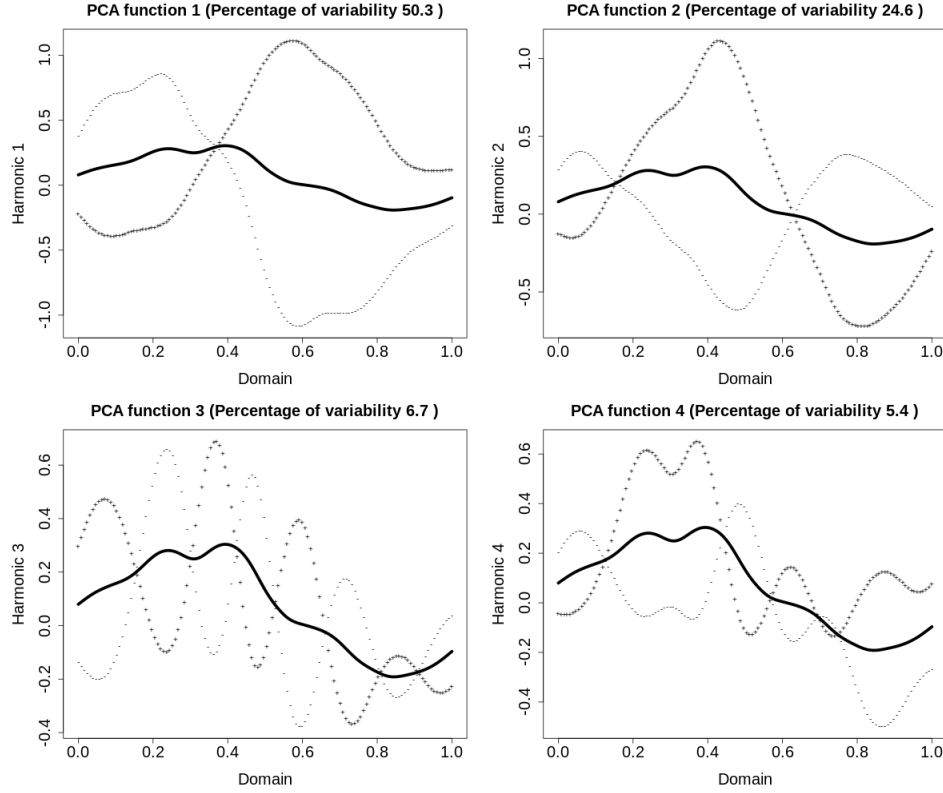

**Fig. S4.** Results of FPCA applied to tsunami emulation data and worst-case scenario time series data at the DART23228 site. The bold line represents the mean function. To illustrate the variation of each principal component curve around the mean function, plus and minus signs indicate two standard deviations. The proportion of variability explained by each principal component function is presented in percentage terms.

explain about 75 percent of the total variance as illustrated in Figure S4. However, even using the first principal component scores derived from the tsunami time series data at the DART23228 observation point to calculate implausibility, it is impossible to identify implausible regions. The reason for this is clearly visualized in Figure S5. At DART23228, the first principal component scores for the emulations and the worst case lay between -0.989 and 0.804 (Figure S5). We do not interpret this range, on its own, as evidence against implausibility. Because the numerator is evaluated in FPCA score coordinates, the denominator must likewise be expressed in the same coordinates before drawing any conclusion. Given such small score differences, we cannot judge whether the implausibility is below the Chebyshev based screening threshold unless the denominator is expressed in the same FPCA score coordinates as the numerator. This means representing emulator uncertainty, observational uncertainty, and model discrepancy in that coordinate system. However, FPCA does not directly propagate the OPE induced predictive



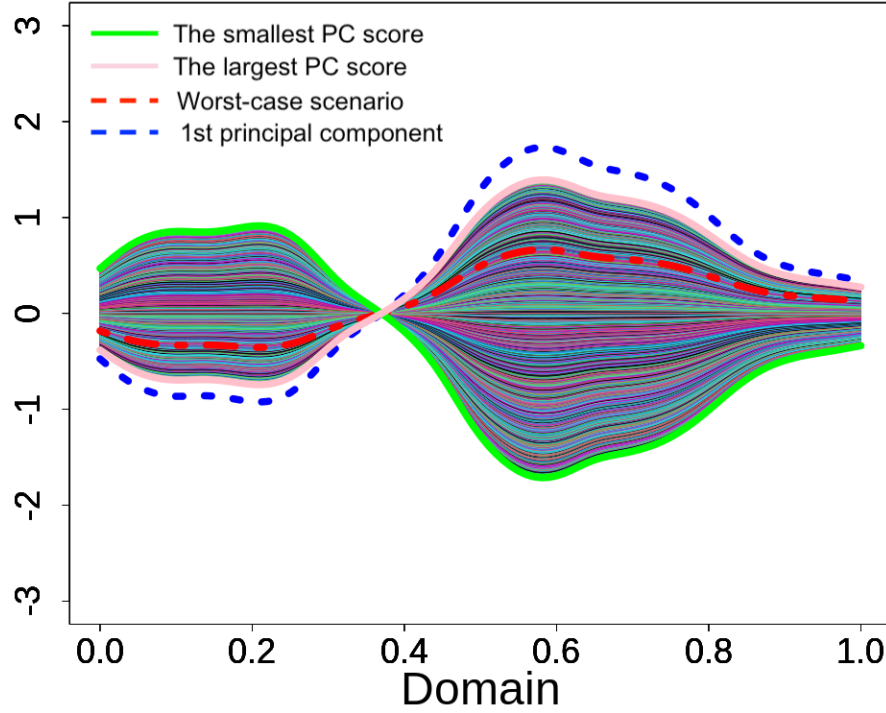

**Fig. S5.** Results of FPCA of one million emulation data at observation point DART23228 during Wave 1, shown against the worst-case scenario (indicated by a red dashed line). The product of the principal component scores and the first eigenfunction represents the first principal component direction of each tsunami time series data. The tsunami time series data with the highest and lowest principal component scores are indicated with thick pink and green lines, respectively. The principal component function is shown as a blue dashed line.

uncertainties into the score coordinates. In practice, this would require computing, for each emulated curve, the uncertainty along the first principal component (and similarly for additional components), which is computationally prohibitive at the scale required for near real time analysis. Consequently, we do not adopt FPCA based implausibility.

### E. Reproducing Kernel Hilbert Space projection

Another strategy is to project infinite dimensional functions into a finite dimensional Reproducing Kernel Hilbert Space (RKHS) (Berlinet & Thomas-Agnan 2011). With a reproducing kernel Hilbert space  $\mathcal{H}_k$  and an orthonormal basis  $\{\phi_i\} \in \mathcal{H}_k$ , each function is represented by the truncated expansion

$$f(t) = \sum_{i=1}^d \lambda_i \phi_i, \quad \lambda_i = \langle f, \phi_i \rangle_{\mathcal{H}_k}, \quad (\text{S10})$$

where  $d$  is the projection dimension. While effective for dimensionality reduction, RKHS projections do not explicitly encode phase information. As with  $L_2$  norms, they primarily reflect amplitude differences, so curves that are out of phase may still be judged close, whereas curves that are in phase but differ in amplitude may be judged far. To address this issue, projecting the differentiated curves of tsunami time series data into the RKHS can be an effective method. This approach allows us to obtain a set of  $d$ -dimensional discrete data,  $\{\lambda'_1, \lambda'_2, \dots, \lambda'_d\}$ . However, there are several challenges associated with this technique that need to be addressed in our research. Practical challenges include choosing the projection dimension  $d$ , selecting an appropriate kernel and bandwidth, and managing the computational burden for large scale comparisons. Moreover, in computing implausibility, if the numerator is computed as a distance in the RKHS coefficient space, the denominator must likewise be expressed in the same coordinates. This includes emulator uncertainty, observational uncertainty, and model discrepancy, and doing so reliably at scale is nontrivial and adds further computational cost.

## F. Random Projection

To address these issues, we evaluate distances via random projection. Random projection preserves pairwise distances in expectation and concentrates with multiple projections, providing a computationally light surrogate for high-dimensional comparisons. This method has been employed in classification (Arriaga et al. 2015, Xie et al. 2016), clustering (Tasoulis et al. 2014, Zhao et al. 2016), and regression analysis (Maillard & Munos 2012, Geppert et al. 2017), demonstrating broad applicability. In our setting, a one dimensional projection is obtained by the inner product  $\langle f(t), h(t) \rangle = \int f(t)h(t)dt$  with a random function  $h$  drawn from a stochastic process such as the Wiener process (Brown 1828), the Ornstein-Uhlenbeck processes (Uhlenbeck & Ornstein 1930), or fractional Brownian motion (Mandelbrot & Van Ness 1968). We use draws from the Wiener process, with the time unit set to the simulation time step, because they are simple to simulate and computationally efficient. To encode phase related information, we also apply random projection to differentiated time series. Since a single projection depends on the draw  $h$ , we compute projections for many independent random functions and use their average as a stable estimate. As shown in Figure S6, averaging 1,000 projections across diverse directions yields stable distance estimates.

## 4. UNCERTAINTY EVALUATION

To perform functional history matching, it is essential to calculate implausibility as seen in Equation 1 in the main paper, which requires the assessment of uncertainty. Generally, this uncertainty can be divided into three sources: those originating from emulators, those due to observational

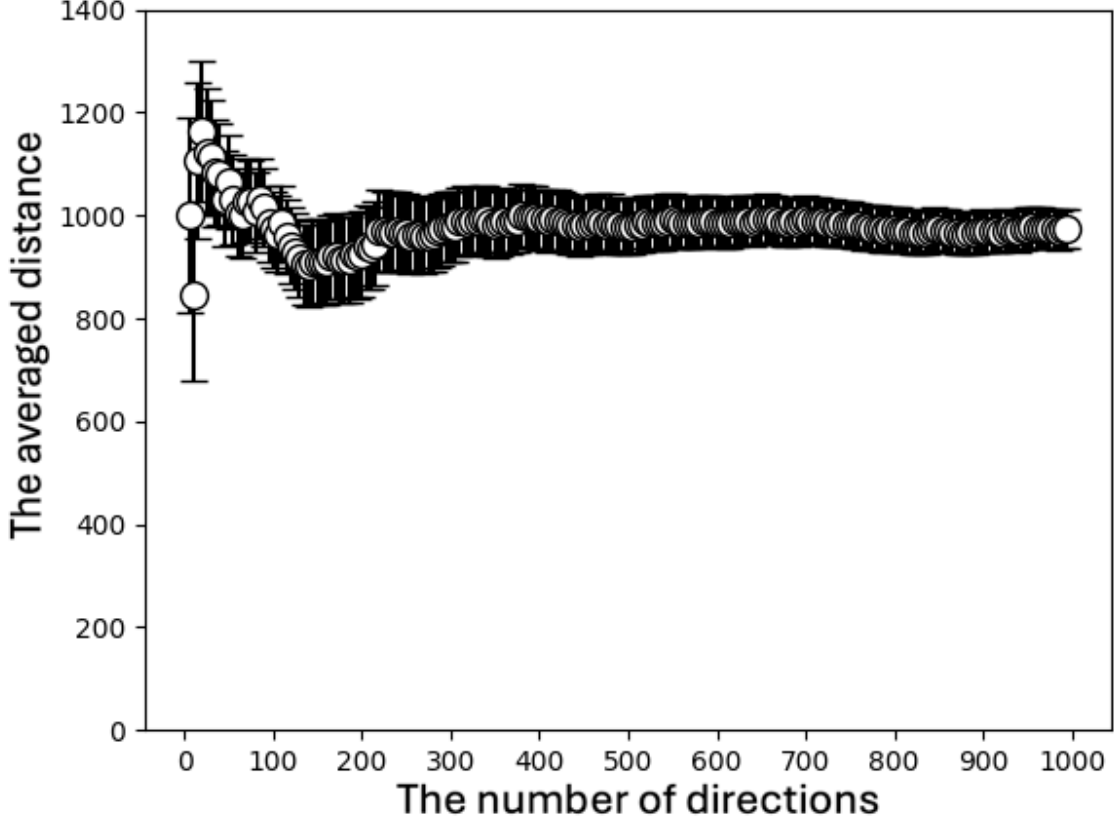

**Fig. S6.** The average distance between an emulation curve and the worst-case scenario curve converges using random projections. The error bars indicate  $\pm\sigma$ .

errors, and those due to model discrepancies. In this study, we construct an emulator using OPE and generate emulated tsunami time series data. Additionally, by differentiating these emulated time series data, we can also emulate the velocity of sea surface fluctuations. Given that OPE uses the NIG framework, the uncertainty in the emulated tsunami time series data can be determined. In this framework, the regression coefficients  $\beta = (\beta_1, \beta_2, \dots, \beta_\nu)$  is modeled as a multivariate normal distribution with a covariance matrix of  $\tau V$ , and the error term  $\varepsilon$  is assumed to follow a Gaussian process. Consequently, given that  $\beta$  and  $\varepsilon$  are independent when conditioned on  $\tau$ , the uncertainty in predictions  $y = G\beta + \varepsilon$  is the sum of these two uncertainties,

$$V[y|\tau] = V[G\beta|\tau] + V[\varepsilon|\tau] = \tau(GVG^T + W), \quad (\text{S11})$$

where  $\tau W = V[\varepsilon]$ . The hyperparameter  $\tau$  is modeled as an inverse gamma distribution with hyperparameters  $(a, d)$ ,

$$\text{IG}(\tau; a, d) = \frac{(d/2)^{a/2}}{\Gamma(a/2)} \tau^{-(1+a/2)} \exp \left\{ -(d/2)\tau^{-1} \right\}. \quad (\text{S12})$$

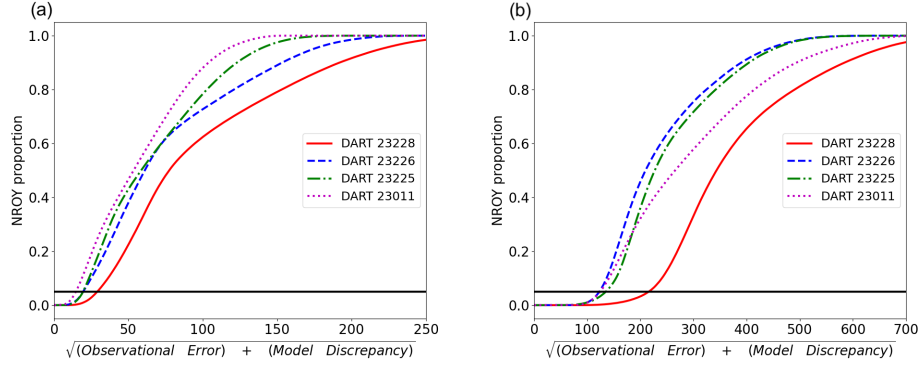

**Fig. S7.** Convergence of the NROY proportion for tsunami time series emulation results and their first derivatives. The horizontal axis shows the square root of observational errors plus model discrepancies. Emulator uncertainty varies across emulations; it is accounted for in the denominator but omitted from the horizontal axis for interpretability. The vertical axis is the NROY proportion.

Here, unlike the conventional notation of the inverse gamma distribution, we use an expression where  $\frac{a}{2}$  and  $\frac{d}{2}$  are inserted into the gamma function and exponential function, respectively, to simplify the notation following the integration of  $\tau$ . Therefore, since  $y$  follows a multivariate normal distribution and its variance is known, by integrating out  $\tau$ , we find that the distribution of  $y$  follows a Student's t-distribution. This procedure remains valid even when updating the distribution shapes of various parameters using observations, asserting that  $y$  still follows a Student's t-distribution. Based on these results, the variance of this t-distribution is used to represent the emulator-derived uncertainty in the calculation of implausibility. Also, in functional history matching for differentiated tsunami time series data, we evaluate the uncertainty of the emulator-derived differentiated curves at a given parameter value by sampling the tsunami time series data 1,000 times with the same parameters, differentiating each sample, and observing the variability across these 1,000 iterations. To quantify the Monte Carlo error of this estimate, we use a delta method approximation: the standard error of the standard deviation based on  $n$  emulator draws is  $SE(\hat{\sigma}) \approx \hat{\sigma} / \sqrt{2(n-1)}$ , so the relative standard error is  $RSE(\hat{\sigma}) \approx 1 / \sqrt{2(n-1)}$  (about 2.2 % for  $n = 1000$ ).

As described in the main paper we have calculated uncertainty based on observational error and model discrepancies using a method that divides the ensemble into  $k$  folds, following the concept of cross-validation. Specifically, this procedure seeks to establish uncertainty under conservative conditions where 5% of the elements in each fold are considered non-implausible. Using this method, it is possible to compute implausibility, thereby distinguishing between

implausible subspace and non-implausible subspace (NROY subspace). One of the methods to validate this new approach is to increase uncertainty and verify whether the proportion of NROY converges to one, as suggested in [McNeall et al. \(2016\)](#). This approach effectively confirms the relationship between uncertainty and NROY subspace as illustrated in Figure S7. In this figure, under the assumptions that observational errors are uniform at the same observation points and that model discrepancies are consistent across all simulations because of the use of the same model, the horizontal axis quantifies the uncertainty stemming from these assumed uniform model discrepancies and observation errors in all emulation curves. Figure S7 varies the square root of the sum of observational error and model discrepancy along the horizontal axis. Emulator uncertainty is included in the implausibility denominator for every emulated curve, but because it differs across curves it is held at its curve specific value and therefore is not shown on the axis. It is important to note that the uncertainty originating from emulation varies slightly among the emulation curves; therefore, a single value cannot be assigned to all curves, and this uncertainty has not been included on the horizontal axis. Also, the NROY ratio is set on the vertical axis.

This diagram illustrates several important points. Firstly, at all observation points, the proportion of NROY smoothly increases as uncertainty is incrementally raised, for both the tsunami time series data and the derivative data. This indicates that the functional emulation and the evaluation of distances between functional data conducted through our method have been appropriately performed. Next, this figure can be interpreted to show which observation points are more likely to classify the parameter space as implausible ([McNeall et al. 2016](#)). From the plot for the original curves, at observation point DART 23228, closest to the MSZ, a larger portion of the parameter space is excluded (resulting in a smaller NROY proportion) compared to the most distant point, DART 23011, even when observational errors and model discrepancies are considered significant. This means that assuming identical values of uncertainty at each observation point, the findings indicate that the nearest point exhibits the smallest proportion of the NROY subspace. Therefore, among these four observation points, the data from DART 23228 can be regarded as the most valuable in terms of applying constraints on the parameter space.

For the derivative curves, the order of the proportion excluded for the same value of uncertainty differs from that of the tsunami time series data. This indicates that the differentiated curves, carrying information about the peak and bottom timing of the time series data, contribute differently to align phases. In other words, when the focus is on the velocity of sea surface changes, each observation point impacts the implausibility in a manner different from when sea surface values are targeted. In this method, when estimating uncertainty originating from observational errors and model discrepancies, a conservative approach is taken by adopting the value where 5% is categorized as NROY. Therefore, we use the uncertainty values derived from

**Table S1.** Square root of the estimated uncertainty (model discrepancy and observational error).

| DART                  | 23228  | 23226  | 23225  | 23011  |
|-----------------------|--------|--------|--------|--------|
| Original curves       | 29.04  | 19.55  | 19.52  | 14.68  |
| Differentiated curves | 215.73 | 122.87 | 135.06 | 124.40 |

each curve's intersection points with this horizontal line in Figure S7. The square root of these uncertainty values in wave 1 is detailed in Table S1.

The usefulness of history matching is reflected in the NROY proportion. If the assumed uncertainties are overly large, the NROY proportion approaches one and little can be ruled out. Conversely, under defensible uncertainty levels, persistent mismatch between emulator and observations can drive the NROY proportion toward zero. Such outcomes indicate potential misspecification in the simulator, the discrepancy, or the prior input ranges and warrant reassessment.

## 5. ESTIMATION AT DART LOCATIONS AND IMPLAUSIBILITY ANALYSIS

Figure 4 in the main paper presents the estimated results of wave 1 only at the observation point DART23228, which is closest to the tsunami off the Makran coast. Similarly, the results for wave 1 at other observation points, DART23226, DART23225, and DART23011, are shown in this supplemental material in Figures S8. These figures illustrate the results of (1) one million emulations, (2) functional history matching applied to tsunami time series data at each observation point, and (3) functional history matching results based on sea surface velocity time series data derived from differentiated tsunami time series data combined with the aforementioned functional history matching results for the tsunami time series. These data are derived from an emulator constructed based on an ensemble using the same set of input parameter values obtained through Latin hypercube sampling as mentioned in the main paper. The emulation results based on randomly assigned parameter values shown on the left cannot be said to accurately estimate the worst-case scenario tsunami data represented by a thick black line. This is a natural outcome because the input values are randomly selected. In the middle of the figure, the selected emulation curves that are physically close to the worst-case scenario curve indicate that the functional history matching is effective. Nevertheless, the fact that curves with peaks at different times from the worst-case scenario are also chosen underscores the necessity of employing

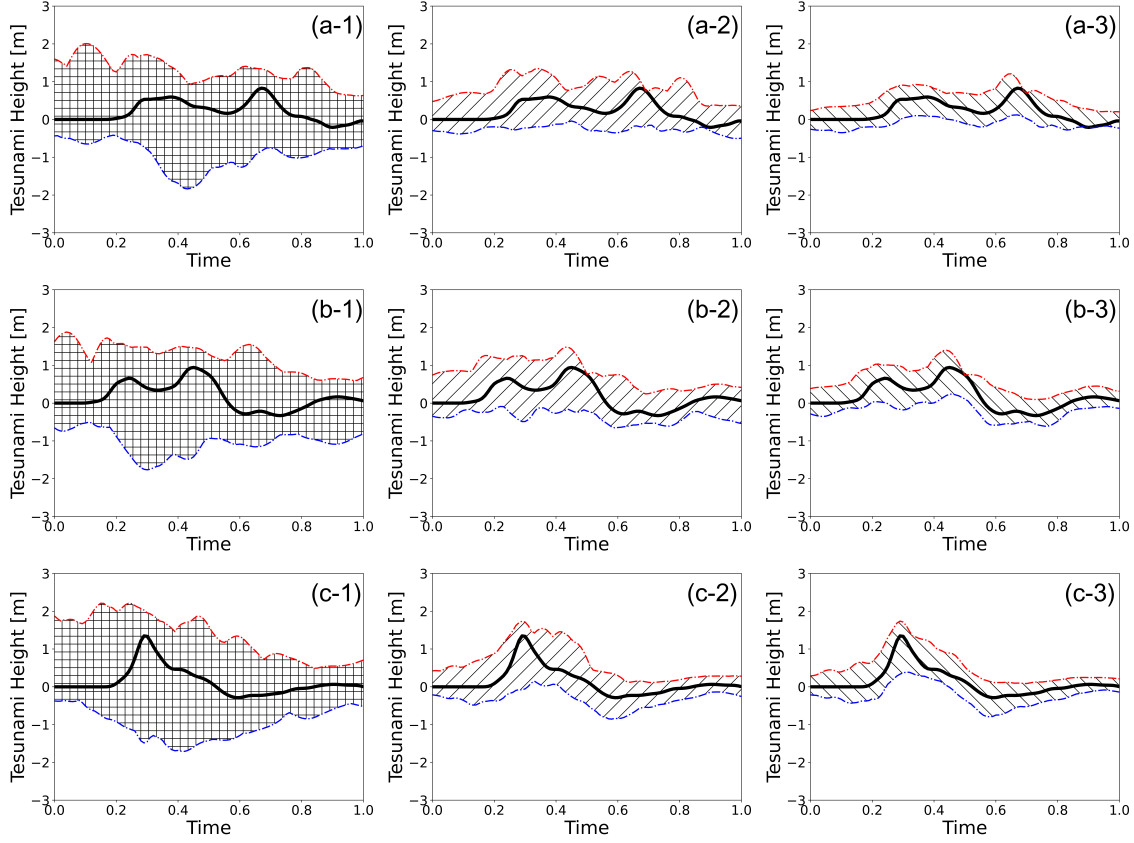

**Fig. S8.** Emulation Results and Parameter Constraints at the DART 23226, 23225, and 23011 observation Location. Panel (a-1): the results of one million emulations, Panel (a-2): the functional history matching result based on tsunami time series data, and Panel (a-3): the functional history matching result based on tsunami time series data and its derivatives for DART 23226. Regarding DART23225 and DART23011, the figures on the second and third levels are equivalent to those in DART23026.

functional data. This observation is because emulation curves deemed close in physical distance to the worst-case scenario time series do not necessarily share the same positions of peaks and troughs. The results of applying functional history matching to both original tsunami time series data and its derivatives, to incorporate the phase information known as sea surface velocity, are shown on the right. It can be verified that the phases are aligned. These results demonstrate the advantages of functional data analysis by showing that, by taking the information from differentiated curves into account, it is possible to select emulation curves that are physically close to the worst-case scenario time series data and aligned in phase.

Generally, implausibility distribution at different observation points possesses distinct char-



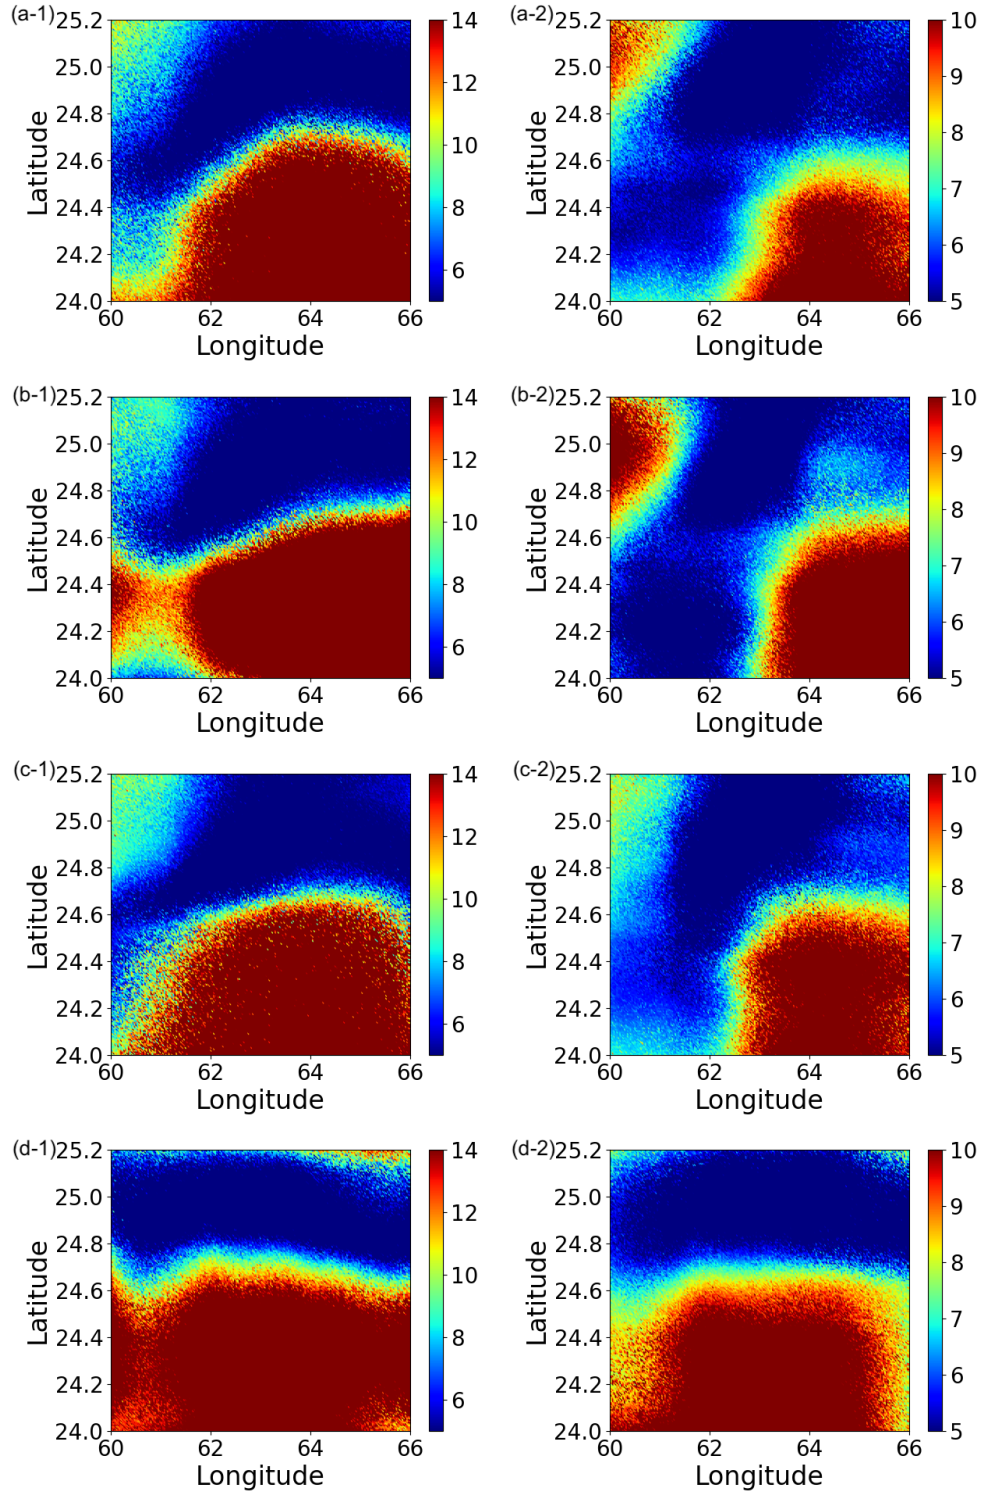

**Fig. S9.** Distribution of Implausibility for tsunami time series data (left) and the derivative curves (right) at observation points 23228 (a-1, a-2), 23226 (b-1, b-2), 23225 (c-1, c-2), and 23011 (d-1, d-2) during wave 1.

acteristics. To demonstrate this, the distribution of implausibility in wave 1 projected onto a two-dimensional space of longitude and latitude is presented in Figure S9. This figure illustrates, for instance, that the distribution of implausibility calculated from tsunami time series data at the DART23228 station closest to the tsunami source (Panel (a-1)) and implausibility derived from tsunami time series data at the farthest DART23011 station (Panel (d-1)) are different. Furthermore, as demonstrated by the implausibility distributions calculated from the tsunami time series data and their derivative curves, which represent the time series data of sea surface change velocity, significant differences exist at DART23228 and DART23226 as depicted in Panel (a-1) and (a-2), and Panel (b-1) and (b-2), respectively.

## 6. INVERSE ESTIMATION, FORECASTING AND COMPARISON.

Our functional history matching approach allows for the inverse estimation of the initial tsunami. In this study, a total of 2,381 parameter sets were selected in wave 1, and 497 sets in wave 2. Given the extensive range of longitude direction within the initial parameter space  $\Theta$ , it is considered challenging to estimate the worst-case scenario tsunami without appropriately selecting a set of parameter values. Figure S10 depicts the inverse estimation of the initial tsunami in the longitude direction at the location where the initial tsunami reaches its highest in the worst-case scenario. As shown in Panel (a), the initial tsunami associated with the set of parameter values constructing the ensemble for the emulator has an average near zero and is bounded by extremely large maximum and minimum values, making it inadequate for accurately estimating the initial tsunami with this data alone. In contrast, the result from wave 1 in Panel (b) shows a reduced range between maximum and minimum values and the estimated average curve closer to the true shape of the initial tsunami. Furthermore, Panel (c) shows that in wave 2 the uncertainty has been reduced and the estimated average shape more closely resembles the worst-case scenario.

Figures S11 displays tsunami forecasting at the observation points 002, 003, and 004 using functional history matching (left) and landmark-based history matching (right). For observation point 002, we examined 90 minutes from 14:30 to 16:00, while for points 003 and 004, it's 120 minutes from 14:00 to 16:00, with the time ranges being transformed to fit within the  $[0, 1]$  interval. The forecasting curves using functional history matching are highly accurate with low amplitude. This result means that, although reducing the parameter space does not always contribute to forecasting accuracy, our methodology effectively narrows down the parameter space to facilitate accurate forecasting.

Regarding landmark-based history matching, we constructed an emulator using Gaussian process regression with a Matérn kernel as expressed in Equation S13, targeting four landmarks:

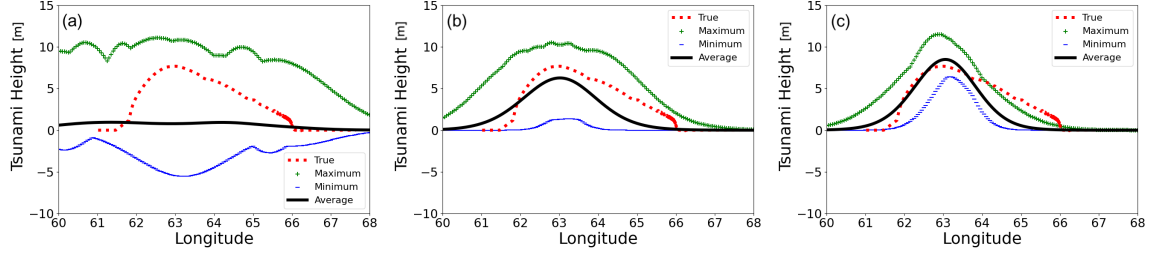

**Fig. S10.** Inverse estimation of the initial tsunami at the maximum height point in longitude direction. The maximum and minimum values of the selected curves are marked with + and – respectively. A bold black line represents the mean value of the selected curves, while a red dotted line shows the worst-case scenario initial tsunami. Panel (a): Represents the initial tsunami used in 100 JAGURS simulations for constructing the ensemble for the emulator. Panel (b): Results of functional history matching in wave1. Panel (c): Results of functional history matching in wave 2.

the maximum and minimum tsunami heights and the elapsed times to reach these extremes. The emulator was trained using the same simulation ensemble used for functional history matching in wave 1.

$$f(x) \sim \mathcal{GP}(m(x), k(x, x')), \quad (\text{S13})$$

where,  $x$  is the input,  $f(x)$  is the output corresponding to  $x$ ,  $m(x)$  is the mean function of the Gaussian process, and  $k(x, x')$  is the covariance function for any two input points  $x$  and  $x'$ . In this study, the input  $x$  consists of five-dimensional parameters: the longitude and latitude at the midpoint of the tsunami's rise and fall, the standard deviations in the longitude and latitude directions, and the tsunami height. The output is a tsunami value such as the maximum of the tsunami time series data. For this analysis, we assume  $m(x) = 0$ . Given a set of training data  $(X, y)$ , the predicted value  $f(x^*)$  at a new input  $x^*$  through Gaussian Process Regression is expressed as follows.

$$f(x^*) | X, y, x^* \sim \mathcal{N}(\mu(x^*), \sigma^2(x^*)) \quad (\text{S14})$$

The predicted mean  $\mu(x^*)$  and variance  $\sigma^2$  of the normal distribution that  $f(x^*)$  follows are expressed as follows.

$$\mu(x^*) = k(x^*, X) [K + \sigma_n^2 I]^{-1} y \quad (\text{S15})$$

$$\sigma^2(x^*) = k(x^*, x^*) - k(x^*, X) [K + \sigma_n^2 I]^{-1} k(X, x^*) \quad (\text{S16})$$

Here,  $K$  denotes the kernel matrix for the training data,  $\sigma_n^2$  represents the variance of the noise, and  $I$  is the identity matrix. Also, this study defines the covariance function using the Matérn

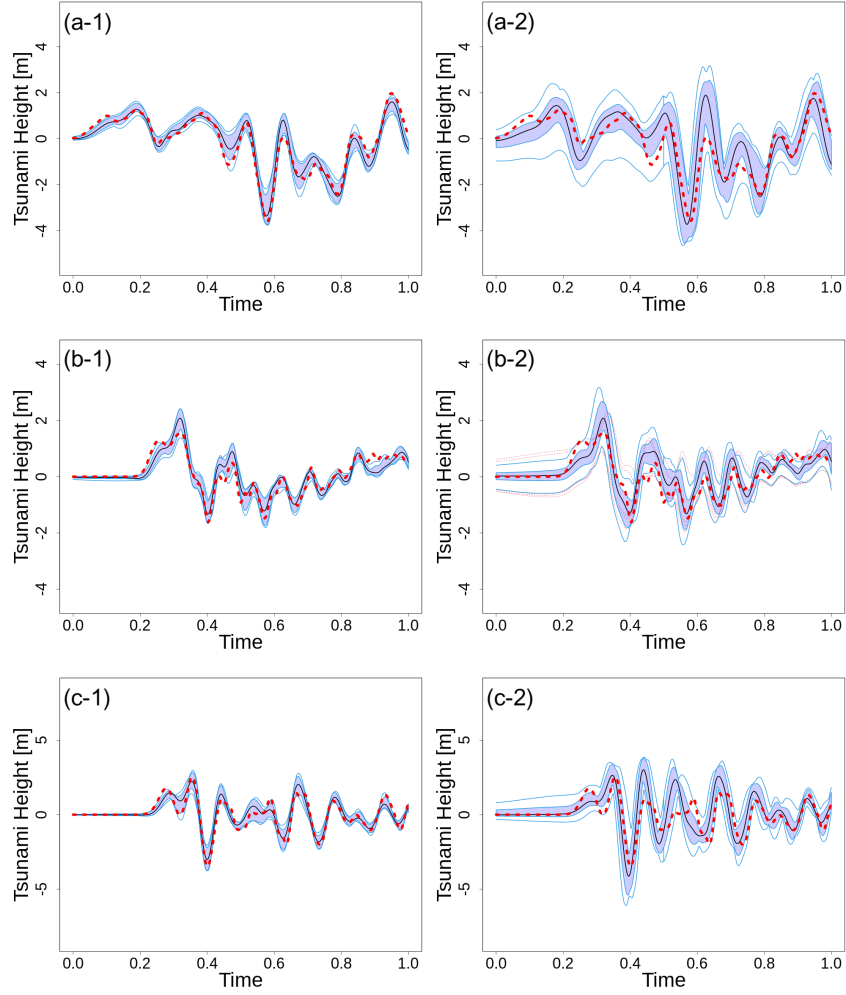

**Fig. S11.** Tsunami forecasting at Mumbai observation points. Panel (a-1), (b-1), and (c-1) are FHM results in wave 2 at 002, 003, and 004 observation points, respectively. Panel (a-2), (b-2), and (c-2) are landmark-based HM results in wave 2.

kernel, as described below.

$$k(x, x') = \frac{2^{1-\nu}}{\Gamma(\nu)} \left( \frac{\sqrt{2\nu} \|x - x'\|}{l} \right)^\nu K_\nu \left( \frac{\sqrt{2\nu} \|x - x'\|}{l} \right), \quad (\text{S17})$$

where  $K_\nu$  represents the modified Bessel function of the second kind,  $\Gamma$  denotes the gamma function, and the value of  $\nu$  is set to 2.5.

Then, we obtained 16 implausibility values  $I_1(\theta), \dots, I_{16}(\theta)$  for each  $\theta$ . Similar to the approach in [Vernon et al. \(2014\)](#), NROY parameter subspace is constructed using the largest implausibility value among 16 calculated measures. After this, the landmark-based history matching method is

**Table S2.** The number of selected curves based on implausibilities targeting the maximum values, minimum values, and elapsed time to reach them at each DART observation point with landmark-history matching in wave 1.

| DART       | 23228   | 23226     | 23225     | 23011     |
|------------|---------|-----------|-----------|-----------|
| Max Height | 845,408 | 1,000,000 | 1,000,000 | 957,115   |
| Min Height | 994,644 | 983,557   | 999,836   | 1,000,000 |
| Max timing | 51,454  | 49,394    | 110,061   | 93,096    |
| Min timing | 53,685  | 31,433    | 89,716    | 304,202   |
| All        | 3,601   | 2,906     | 16,259    | 48,289    |

repeated using the shrunk parameter subspace  $\Theta_1$ . It is observed that the maximum heights of the tsunamis near Mumbai are often overestimated, and the amplitude of the estimated tsunami is larger compared to those from our functional history matching approach. In calculating implausibility, we consider only the uncertainty derived from the aforementioned Gaussian process regression as the most extreme assumption. This condition can be considered the assumption that allows for the highest evaluation of implausibility, as evidenced by the reduction in implausibility values when additional uncertainties such as observational errors or model discrepancy are incorporated, thus enabling the greatest exclusion of parameter subspace.

Nevertheless, the outcomes of performing history matching independently for maximum and minimum values, and their arrival times at each DART observation site, as shown in Table S2, did not function efficiently. Despite considering only the uncertainty originating from Gaussian process regression, which was thought to be extremely advantageous for reducing the NROY subspace, the history matching for discrete data did not function properly. This indicates that using only these specific observation points for the time series data is insufficient.

## 7. VIRTUAL OBSERVATION POINT

By placing a hypothetical observation point at the location indicated by the black circle in Figure S1, we examine the changes that occur compared to functional history matching conducted only with the existing four DART observation points. This aims to understand the impact of constructing the NROY parameter subspace when adding an observation point on the opposite

side, as opposed to having all observation points in the same direction from the tsunami source. Figure S12 includes the results of the initial tsunami inverse-estimation at the locations recording the maximum and minimum tsunami heights in the worst-case scenario, at (63.017, 24.366) and (63.623, 25.311) respectively. Comparisons between Panel (a) and (b), as well as Panel (c) and (d), clearly demonstrate a reduction in the NROY subspace in low-longitude regions, indicating that even a single virtual observation point can be highly effective.

To assess the specific effects on the NROY parameter subspace shrinkage caused by this virtual observation point, Figure S13 presents violin plots showing the non-implausible regions for each parameter, where it is evident that there is a significant restriction in the longitude and the tsunami height. It can also be seen that there is a minor contraction in the  $S_{xx}$  direction. One possible reason for observing such a phenomenon is that tsunamis located at low longitude need to be exceptionally large to replicate the worst-case scenarios at the four DART observation points. However, it is hypothesized that the virtual observation point on the opposite side of the DART points has eliminated such large tsunamis.

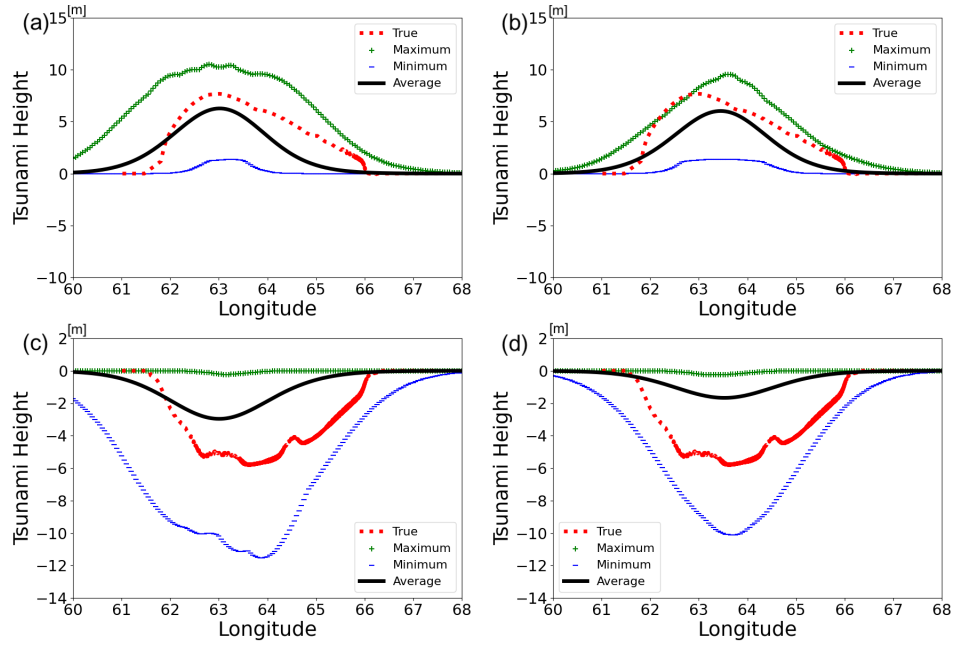

**Fig. S12.** Comparison of the estimation of initial tsunami (longitude direction) using only four DART observation points, Panel (a) and (c), versus adding a virtual observation point, Panel (b) and (d), in wave 1. Panel (a) and (b): The initial tsunami estimation at the location of the highest tsunami height under the worst-case scenario. Panel (c) and (d): The initial tsunami estimation at the location of the lowest tsunami height under the worst-case scenario.

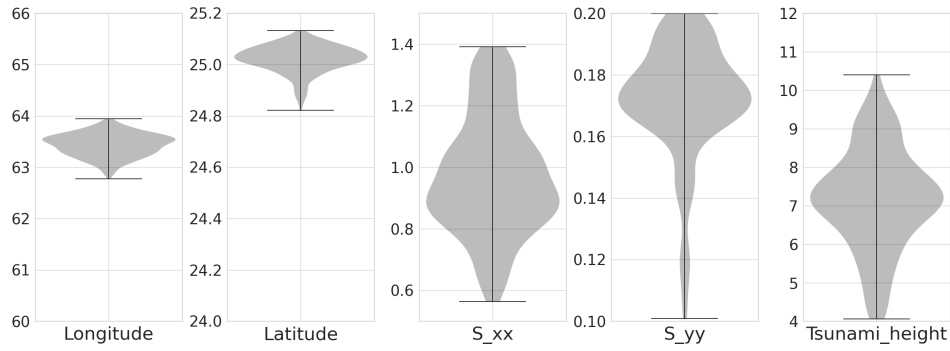

**Fig. S13.** Violin plots with an additional virtual observation point added to the four DART observation points in wave 1.



## REFERENCES

- Alt, H. & Godau, M. (1995), 'Computing the fréchet distance between two polygonal curves', *International Journal of Computational Geometry & Applications* 5(01n02), 75–91.
- Arriaga, R. I., Rutter, D., Cakmak, M. & Vempala, S. S. (2015), 'Visual categorization with random projection', *Neural computation* 27(10), 2132–2147.
- Baba, T., Allgeyer, S., Hossen, J., Cummins, P. R., Tsushima, H., Imai, K., Yamashita, K. & Kato, T. (2017), 'Accurate numerical simulation of the far-field tsunami caused by the 2011 tohoku earthquake, including the effects of boussinesq dispersion, seawater density stratification, elastic loading, and gravitational potential change', *Ocean Modelling* 111, 46–54.
- Baba, T., Takahashi, N., Kaneda, Y., Ando, K., Matsuoka, D. & Kato, T. (2015), 'Parallel implementation of dispersive tsunami wave modeling with a nesting algorithm for the 2011 tohoku tsunami', *Pure and Applied Geophysics* 172, 3455–3472.
- Berlinet, A. & Thomas-Agnan, C. (2011), *Reproducing kernel Hilbert spaces in probability and statistics*, Springer Science & Business Media.
- Brankovic, M., Buchin, K., Klaren, K., Nusser, A., Popov, A. & Wong, S. (2020), (k, l)-medians clustering of trajectories using continuous dynamic time warping, in 'Proceedings of the 28th International Conference on Advances in Geographic Information Systems', pp. 99–110.
- Brown, R. (1828), 'Xxvii. a brief account of microscopical observations made in the months of june, july and august 1827, on the particles contained in the pollen of plants; and on the general existence of active molecules in organic and inorganic bodies', *The philosophical magazine* 4(21), 161–173.
- Ferreira, L. & Hitchcock, D. B. (2009), 'A comparison of hierarchical methods for clustering functional data', *Communications in Statistics-Simulation and Computation* 38(9), 1925–1949.
- Geppert, L. N., Ickstadt, K., Munteanu, A., Quedenfeld, J. & Sohler, C. (2017), 'Random projections for bayesian regression', *Statistics and Computing* 27, 79–101.
- Gopinathan, D., Heidarzadeh, M. & Guillas, S. (2021), 'Probabilistic quantification of tsunami current hazard using statistical emulation', *Proceedings of the Royal Society A* 477(2250), 20210180.
- Hall, P., Müller, H.-G. & Wang, J.-L. (2006), 'Properties of principal component methods for functional and longitudinal data analysis', *The Annals of Statistics* 34(3), 1493 – 1517.  
URL: <https://doi.org/10.1214/0090536060000000272>
- Hitchcock, D. B., Casella, G. & Booth, J. G. (2006), 'Improved estimation of dissimilarities by presmoothing functional data', *Journal of the American Statistical Association* 101(473), 211–222.
- James, G. M. & Sugar, C. A. (2003), 'Clustering for sparsely sampled functional data', *Journal of the American Statistical Association* 98(462), 397–408.
- Karhunen, K. (1947), 'Under lineare methoden in der wahr scheinlichkeitsrechnung', *Annales Academiae Scientiarum Fennicae Series A1: Mathematica Physica* 47.
- Loeve, M. (1948), 'Functions aleatoires du second ordre', *Processus stochastique et mouvement*

- Brownien* pp. 366–420.
- Maillard, O. & Munos, R. (2012), ‘Linear regression with random projections’, *Journal of Machine Learning Research* **13**(1), 2735–2772.
- Mandelbrot, B. B. & Van Ness, J. W. (1968), ‘Fractional brownian motions, fractional noises and applications’, *SIAM review* **10**(4), 422–437.
- Marron, J. S., Ramsay, J. O., Sangalli, L. M. & Srivastava, A. (2015), ‘Functional data analysis of amplitude and phase variation’, *Statistical Science* pp. 468–484.
- McNeall, D., Williams, J., Booth, B., Betts, R., Challenor, P., Wiltshire, A. & Sexton, D. (2016), ‘The impact of structural error on parameter constraint in a climate model’, *Earth System Dynamics* **7**(4), 917–935.
- Ramsay, J. O. & Silverman, B. W. (2005), *Fitting differential equations to functional data: Principal differential analysis*, Springer.
- Rougier, J. (2008), ‘Efficient emulators for multivariate deterministic functions’, *Journal of Computational and Graphical Statistics* **17**(4), 827–843.
- Sakoe, H. & Chiba, S. (1978), ‘Dynamic programming algorithm optimization for spoken word recognition’, *IEEE transactions on acoustics, speech, and signal processing* **26**(1), 43–49.
- Tasoulis, S., Cheng, L., Välimäki, N., Croucher, N. J., Harris, S. R., Hanage, W. P., Roos, T. & Corander, J. (2014), Random projection based clustering for population genomics, in ‘2014 IEEE international conference on big data (big data)’, IEEE, pp. 675–682.
- Tokushige, S., Inada, K. & Yadohisa, H. (2003), ‘8. functional data analysis dissimilarity and related methods for functional data’, *Journal of the Japanese Society of Computational Statistics* **15**(2), 319–326.
- Uhlenbeck, G. E. & Ornstein, L. S. (1930), ‘On the theory of the brownian motion’, *Physical review* **36**(5), 823.
- Vernon, I., Goldstein, M. & Bower, R. (2014), ‘Galaxy formation: Bayesian history matching for the observable universe’, *Statistical science* pp. 81–90.
- Xie, H., Li, J., Zhang, Q. & Wang, Y. (2016), ‘Comparison among dimensionality reduction techniques based on random projection for cancer classification’, *Computational biology and chemistry* **65**, 165–172.
- Zhao, K., Alavi, A., Wiliem, A. & Lovell, B. C. (2016), ‘Efficient clustering on riemannian manifolds: A kernelised random projection approach’, *Pattern Recognition* **51**, 333–345.
